# Supplementary material for: Helping Hands: An Object-Aware Ego-Centric Video Recognition Model
Source: arXiv:2308.07918 source file (2023-08-15)
Supplement: Supplementary file 2 [file ekmir_update.tex]

\begin{table}[h]
\centering

\resizebox{\linewidth}{!}{%
\begin{tabular}{cccccccccc}
\hline
\multirow{3}{*}{\textbf{Method}} & \multirow{3}{*}{\textbf{Backbone}} & \multirow{3}{*}{\textbf{\begin{tabular}[c]{@{}c@{}}Batch\\ Size\end{tabular}}} & \multirow{3}{*}{\textbf{\begin{tabular}[c]{@{}c@{}}Object\\ Aware\end{tabular}}} & \multicolumn{6}{c}{\textbf{EK100-MIR}}                                                        \\
                                 &                                    &                                                                                &                                                                                  & \multicolumn{3}{c}{mAP}                       & \multicolumn{3}{c}{nDCG}                      \\
                                 &                                    &                                                                                &                                                                                  & V-T           & T-V           & Avg           & V-T           & T-V           & Avg           \\ \hline
\multicolumn{10}{c}{\textbf{Using our resized videos}}                                                                                                                                                                                                                                                                            \\ \hline
LaViLa                           & TSF-L                              & 1024                                                                           & N                                                                                & 39.0          & 32.0          & 35.5          & 35.3          & 32.8          & 34.0          \\ \hline
Ours                             & TSF-L                              & 128                                                                            & N                                                                                & 38.9          & 30.5          & 34.5          & 36.1          & 32.9          & 34.4          \\
Ours                             & TSF-L                              & 128                                                                            & Y                                                                                & \textbf{40.9} & \textbf{31.1} & \textbf{36.0} & \textbf{38.2} & \textbf{34.8} & \textbf{36.5} \\ \hline
\multicolumn{10}{c}{\textbf{Using resized videos provided by LaViLa~\cite{zhao2022lavila}}}                                                                                                                                                                                                                                                             \\ \hline
LaViLa                           & TSF-L                              & 1024                                                                           & N                                                                                & 40.0          & 32.2          & 36.1          & 36.1          & 33.2          & 34.6          \\ \hline
Ours                             & TSF-L                              & 128                                                                            & N                                                                                & 39.5          & 30.6          & 35.1          & 37.9          & 34.7          & 36.3          \\
Ours                             & TSF-L                              & 128                                                                            & Y                                                                                & \textbf{41.5} & \textbf{32.3} & \textbf{36.9} & \textbf{38.6} & \textbf{35.4} & \textbf{37.0} \\ \hline
\end{tabular}%
}
\vspace{1mm}
\caption{\textbf{Investigation on performance gap from data-loading on EK100-MIR.} We report both the results from our resized videos and from the resized videos provided by LaViLa~\cite{zhao2022lavila}, with other implementation details remaining the same. Our model outperforms the SOTA model LaViLa in both cases.}
\label{tab:ek-mir_upated}
\end{table}
