# Supplementary material for: Helping Hands: An Object-Aware Ego-Centric Video Recognition Model
Source: arXiv:2308.07918 source file (2023-08-15)
Supplement: Supplementary file 3 [file viz.tex]

% \section{Visualization}
% The attention map does not seem to reflect the localization of objects very well, some examples here: \url{https://docs.google.com/presentation/d/13CHq55APYLv-O16LFSE4U1NVj82odsnxERH0XP5gCrk/edit?usp=sharing}
